# Supplementary material for: Automated Evaluation of Retrieval-Augmented Language Models with Task-Specific Exam Generation
Source: arXiv:2405.13622 source file (2024-05-22)
Supplement: Supplementary file 1 [file tasks.tex]

\section{Tasks Granular Analysis Results}
\label{sec:granular}

\begin{figure}[htpb]
    \centering
    \includegraphics[width=\linewidth]{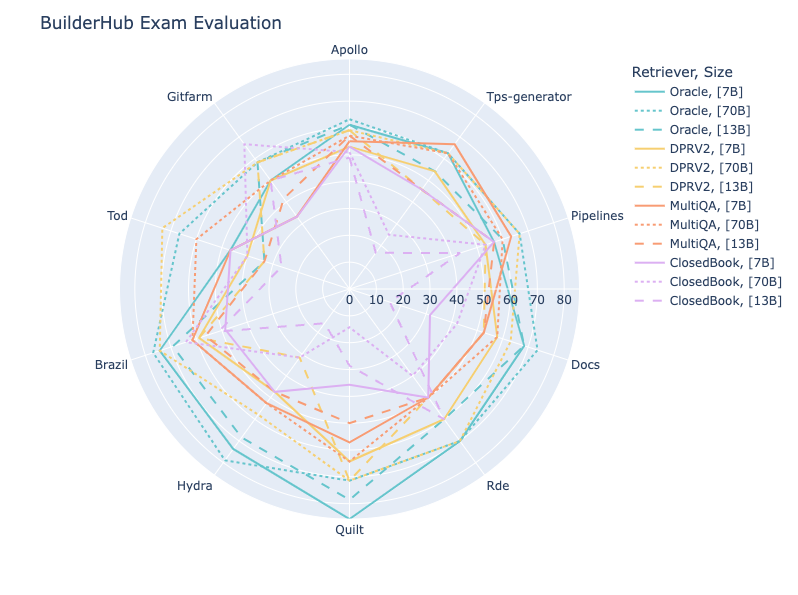}
    \caption{Granular Exam Evaluation for BuilderHub Task \textbf{This is to illustrate and will be removed as AWS confidential data}}
    \label{fig:bh}
\end{figure}

\begin{figure}[htpb]
    \centering
    \includegraphics[width=\linewidth]{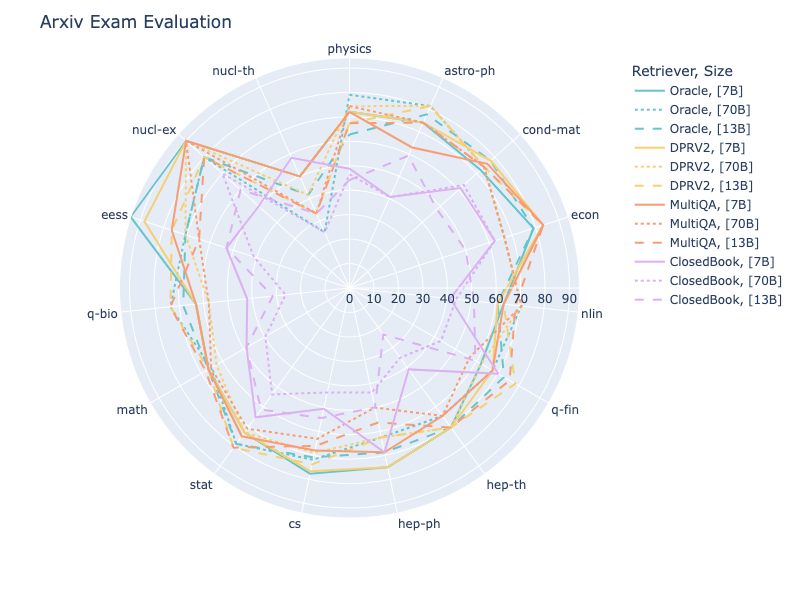}
    \caption{Granular Exam Evaluation for Arxiv Task}
    \label{fig:arxiv}
\end{figure}
